# Supplementary material for: Tuning intraband and interband transition rates via excitonic correlation in low-dimensional semiconductors
Source: arXiv:1806.00595 ancillary file (2018-06-02)
Supplement: Supplementary file 1 [file intraband_v12_supp.pdf]

# Supplemental Material for "Tuning intraband and interband transition rates via excitonic correlation in low-dimensional semiconductors"

Josep Planelles,† Alexander W. Achtstein ,*,‡ Riccardo Scott,‡ Nina Owschimikow,‡ Ulrike Woggon,‡ and Juan I. Climente*,†

†*Departament de Química Física i Analítica, Universitat Jaume I, E-12080, Castelló de la Plana, Spain*

‡*Institute of Optics and Atomic Physics, Technical University of Berlin, Strasse des 17. Juni 135, 10623 Berlin, Germany*

E-mail: achtstein@tu-berlin.de; climente@uji.es

# Size dependence of interband, intraband and inter-valence-band transition matrix elements

Here we give more details and some explicit derivations of the size dependence of transition matrix elements in 2D nanoplatelets and 1D nanorods, with and without exciton correlation. The comparison between the two cases allows us to infer the general case of cuboids with $N$ weakly confined dimensions ($N = 1, 2, 3$), in Table 1 of the main text.

## 2D Nanoplatelets

### Interband matrix element

Let us consider first the interband transition between the filled valence band state $|0\rangle$ and an uncorrelated (independent particle, IP) e-h state $|i\rangle$:

$$\langle i|\mathbf{p}|0\rangle_{IP} \propto N^i_{IP}\langle\Phi^i_{IP}|\delta(\mathbf{r}_e - \mathbf{r}_h)|0\rangle. \quad (1)$$

where we have omitted the Bloch part of the wave function because its matrix element does not scale with the size of the nanostructure. The envelope normalization factor $N^i_{IP} \propto V^{-1}$, as seen in Eq. (3) of the main text, while $\langle\Phi^i_{IP}|\delta(\mathbf{r}_e - \mathbf{r}_h)|0\rangle \propto V$ (since $\langle\Phi^i_{IP}|\delta(\mathbf{r}_e - \mathbf{r}_h)|0\rangle = \int_{-L/2}^{L/2}\prod_i^3 \cos^2 kx_i dx_i \propto L^3 \equiv V$). Therefore, for IP states, $\langle i|\mathbf{p}|0\rangle_{IP} \propto V^0$.

If the arrival state is formed by a correlated exciton, then:

$$\langle i|\mathbf{p}|0\rangle_{corr} \propto N^i_{corr}\langle\Phi^i_{IP}|\delta(\mathbf{r}_e - \mathbf{r}_h)|0\rangle. \quad (2)$$

because the Slater correlation factor, $\Phi^i_{corr}$, becomes unity for $\mathbf{r}_e = \mathbf{r}_h$. Again, $\langle\Phi^i_{IP}|\delta(\mathbf{r}_e - \mathbf{r}_h)|0\rangle \propto V$, but now $N^i_{corr} \propto V^{-1}\sqrt{A/A_X}$, as can be seen in Eq. (4) of the main text. Therefore, $\langle i|\mathbf{p}|0\rangle_{corr} \propto \sqrt{A/A_X}$. In other words, exciton correlation enhances the e-h overlap by a factor $(\sqrt{L/a_B})^2$: $\langle i|\mathbf{p}|0\rangle_{corr} \propto \langle i|\mathbf{p}|0\rangle_{IP}(\sqrt{L/a_B})^2$.

**Intraband matrix element**

These are electron-electron or hole-hole transitions within a same band. If both initial ($|i\rangle$) and final ($|f\rangle$) states are IP states,

$$\langle i|\mathbf{p}|f\rangle_{IP-IP} = \langle \Phi^i_{IP,n}|\mathbf{p}|\Phi^f_{IP,n}\rangle. \tag{3}$$

where $\Phi^f_{IP,n} = N^f_{IP}\,\Phi^f_{IP}$ and $\Phi^i_{IP,n} = N^i_{IP}\,\Phi^i_{IP}$ are normalized wave functions of a cuboidal quantum box. We label $x_1, y_1, z_1$ the electron coordinates, $x_2, y_2, z_2$ the hole ones, and take for example the case of $p_{x_2}$ (derivative $d/dx_2$). An equivalent result is obtained for other in-plane coordinates. We assume that $\Phi^i_{IP,n}$ and $\Phi^f_{IP,n}$ only differ on the $x_2$ part (otherwise the integral is zero). Then we have the integral:

$$\int \Phi^i_{IP,n}\,\frac{d}{dx_2}\,\Phi^f_{IP,n} dx_2 = \frac{2}{L}\int_{-L/2}^{L/2} \cos kx_2 \frac{d}{dx_2}\sin k' x_2\; dx_2 \propto k'. \tag{4}$$

where we have assumed different parity for $\Phi^i_{IP,n}$ and $\Phi^f_{IP,n}$, as otherwise the integral is zero.[1] In the directions other than $x_2$, the integrals are just the norm of normalized functions, and hence do not depend on size. Thus, $\langle f|\mathbf{p}|i\rangle_{IP-IP} \propto k'$. As discussed in the main text, $k'$ depends on the size not only through the $1/L$ term, but also through the quantum number $n'$, which may vary with the size of the nanostructure.

Next, we consider $\Phi^i$ to be correlated and $\Phi^f$ an IP function. Again, we calculate $d/dx_2$ and assume different parity for initial and final functions. In addition to the correlation and normalization factors, we consider that initial and final functions difference is $\cos kx_2$ vs.

[1] In the problem of a particle in a box centered at the origin, the odd functions are $\cos \frac{n\pi}{L}\,x$ with $n$ odd and the even functions are $\sin \frac{n\pi}{L}\,x$ with $n$ even. For example, in the above integral, we may consider $k = \pi/L$, $k' = 2n\pi/L$.

$\sin k' x_2$: After integrating along $z_1$ and $z_2$ direction:

$$
\begin{aligned}
\Phi^i_{corr,n} &= N^i_{corr,\perp} \cos kx_1 \cos kx_2 \cos ky_1 \cos ky_2 e^{-a\sqrt{(x_1-x_2)^2+(y_1-y_2)^2}}, &(5)\\
N^i_{corr,\perp} &= \frac{\sqrt{32/\pi}}{L}\left(\frac{1}{a^2} + \frac{a}{(a^2+k^2)^{3/2}} + \frac{1}{4}\frac{a}{(a^2+2k^2)^{3/2}}\right)^{-1/2}, &(6)\\
\Phi^f_{IP,n} &= N^f_{IP,\perp} \cos kx_1 \sin k'x_2 \cos ky_1 \cos ky_2, &(7)\\
N^f_{IP,\perp} &= \frac{4}{L^2}, &(8)
\end{aligned}
$$

where $a = 1/a_B$, and we have resorted to Eq. (13) of Ref. 1 for the normalization coefficient of the correlated particle. Notice that, for large $L$, $k \ll a$ and then $N^i_{corr,\perp} \propto a/L = 1/(L\, a_B)$. We deal now with the integral,

$$
\begin{aligned}
&\langle \Phi^i_{corr,n} | \frac{d}{dx_2} | \Phi^f_{IP,n} \rangle = \\
&ct.\, \frac{a}{L^3} \int_{-L/2}^{L/2} \cos^2 kx_1 \cos^2 ky_1 \cos^2 ky_2 \cos kx_2 \frac{d \sin k'x_2}{dx_2}\, e^{-a\sqrt{(x_1-x_2)^2+(y_1-y_2)^2}}\, dv
\end{aligned}
\qquad (9)
$$

where $ct.$ is a size-independent constant. The presence of the fast decaying exponential function and a large value of $L$ allows extending the limits of the integral up to infinity without a sensitive change of the integral value.[1] Next, we carry out the following change of variables:

$$
\begin{aligned}
&k' \cos kx_2 \cos k'x_2 = k' \frac{1}{2}\left[\cos(k+k')x_2 + \cos(k'-k)x_2\right] &(10)\\
&\cos^2 ky_2 = (1 + \cos 2ky_2)/2 &(11)
\end{aligned}
$$

This leads to four integrals, all of them with the same $L$-dependence. Let us see the simplest one originated by the term: $\frac{1}{2}k'\frac{1}{2}\cos\tilde{k}x_2$, with $\tilde{k} = k + k'$. We introduce a new change of variables: $\bar{x}_2 = x_2 - x_1$, $\bar{y}_2 = y_2 - y_1$ so that inner $(x_2, y_2)$ double integral becomes:

$$
I_2 = \iint_{-\infty}^{\infty} \cos(2\tilde{k}\bar{x}_2 + 2\tilde{k}x_1) e^{-a\sqrt{\bar{x}_2^2+\bar{y}_2^2}} d\bar{x}_2 d\bar{y}_2 \qquad (12)
$$

similar to Eq. (77) in Ref. 1. Then,

$$I_2 = ct. \frac{a}{(a^2+\tilde{k}^2)^{3/2}} \cos 2\tilde{k}x_1 \tag{13}$$

So that the total integral results:[2]

$$\begin{aligned}\langle \Phi^i_{corr,n}|\frac{d}{dx_2}|\Phi^f_{IP,n}\rangle &= ct. \frac{a}{L^3}\, k' \frac{a}{(a^2+\tilde{k}^2)^{3/2}} \int_{-L/2}^{L/2} \cos^2 kx_1 \cos 2\tilde{k}x_1 \int_{-L/2}^{L/2} \cos^2 ky_1 dx_1 dy_1 \\ &\propto \frac{k'}{L^3}\frac{a^2}{(a^2+\tilde{k}^2)^{3/2}}\, L\, L \approx k'\frac{1}{a\,L} = k'(\sqrt{\frac{a_B}{L}})^2 \end{aligned} \tag{14}$$

where we have taken into account that $a = 1/a_B$ and, for large $L$, $\tilde{k} \to 0$. In short, we see that $\langle f|\mathbf{p}|i\rangle_{IP-corr} \propto \langle f|\mathbf{p}|i\rangle_{IP-IP}(\sqrt{\frac{a_B}{L}})^2$.

The case of correlated intermediate and final states is similar to that we have just seen, because the two correlation factors can be merged into a single one with exponent $a$ replaced by $a+a'$. The momentum operator splits the integral in two. The first one (derivative of the sine) is formally identical to Eq. (9). The second one (derivative of the exponential) vanishes in the limit of large $L$. Yet, upon replacing $N^f_{IP,\perp}$ by $N^f_{corr,\perp}$, the dimension dependence changes (cf. Eqs. (6) and (8)). One finally obtains $\langle f|\mathbf{p}|i\rangle_{corr-corr} \propto k'\, a_B\, a'_B/(a_B+a'_B)^2$.

### Inter-valence-band matrix element

Here we consider transitions between different valence subbands, such as HH to LH or SOH. The general form of the matrix elements is:

$$\langle i|f\rangle \propto N^i\, N^f \langle \Phi^i_{IP}\, \Phi^i_{corr}|\Phi^f_{IP}\, \Phi^f_{corr}\rangle. \tag{15}$$

[2] Please note that at this point the integrand does not contain the exponential function. Then, we keep the integral limits at $\pm L/2$.

where we have omitted the Bloch part because it is size-independent. For transitions between two IP states, it is immediate that the transition is forbidden by envelope function orthogonality unless $|i\rangle$ and $|f\rangle$ have the same quantum numbers (because we consider a cuboidal box of infinite confinement potential, the envelope function does not depend on the masses, which may differ for different subbands), and it is one (size-independent scalar) otherwise because the functions are normalized.

For transitions from a correlated to an IP exciton, we obtain size dependences by analyzing the case where initial and final states have the same IP quantum numbers (Eqs. (5-8). Similar results are expected for other states, but matrix elements will likely be smaller due to quasi-orthogonalities. The matrix element derivation is then similar to that of intraband transitions, except that there is no derivative in the envelope part. Using analogous changes of variable and extension of integral limits, from $\pm L/2$ to infinity, one obtains:

$$\langle i|f\rangle \propto N^i_{corr}\, N^f_{IP} \langle \Phi^i_{IP}\, \Phi^i_{corr} | \Phi^f_{IP} \rangle = \sqrt{18\pi}\, \frac{a_B}{L}. \tag{16}$$

and for transitions between two correlated states:

$$\langle i|f\rangle \propto N^i_{corr}\, N^f_{corr} \langle \Phi^i_{IP}\, \Phi^i_{corr} | \Phi^f_{IP}\, \Phi^f_{corr} \rangle = 4\, \frac{a_B\, a'_B}{(a_B + a'_B)^2}. \tag{17}$$

where $a_B$ is Bohr radius of $|i\rangle$ and $a'_B$ that of $|f\rangle$. It can be seen that the matrix element has a maximum for $a_B = a'_B$ (i.e., the states in the two subbands have identical correlation strength) and decreases otherwise. Because the (ground state, 2D limit) effective exciton Bohr radius (in atomic units) is $a_B = \varepsilon_r/2\mu$, with $\varepsilon_r$ the relative dielectric constant and $\mu$ the exciton reduced mass, in general inter-VB transitions will be faster the closer the effective masses of the different subbands. The fact that $a_B \approx a'_B$ maximizes the transition matrix element can be interpreted because then HH and LH (assuming e.g. these are the hole subbands of $|i\rangle$ and $|f\rangle$) have similar orbitals around the exciton electron.

One can see from the previous equations that explicit size dependence only appears for

transitions from IP to correlated states, but not for cases where the correlation strength of $|i\rangle$ and $|f\rangle$ is similar (IP-IP or correlated to correlated). Besides, the size dependence in Eq. (16) is the inverse of that found in valence-to-conduction band transitions, Eq. (2).

## 1D Nanowires

In nanowires the correlation factor is one-dimensional. The wave function along the wire axis ($z$-direction) reads:

$$
\begin{aligned}
\Phi^m_{corr,n} &= N^m_{corr,\|} \cos kz_1 \cos kz_2 e^{-a|z_1-z_2|}, & (18)\\
N^m_{corr,\|} &= \sqrt{\frac{2}{L}}\sqrt{\frac{8a\,(a^2+k^2)}{6a^2+4k^2}} & (19)\\
,\Phi^m_{IP,n} &= N^m_{IP,\|} \cos kz_1 \cos kz_2, & (20)\\
N^m_{IP,\|} &= \frac{2}{L}. & (21)
\end{aligned}
$$

where the $N_{corr,\|}$ is taken from Eq. (33) of Ref. 1. For long wires, $k \ll a$ and $N^m_{corr,\|} \propto \sqrt{a/L} = 1/\sqrt{L\,a^m_B}$.

### Interband matrix element

Interband transition elements can be understood with the same reasoning as in Eq. (2). $\langle \Phi^m_{IP}|\delta(\mathbf{r}_e - \mathbf{r}_h)|0\rangle \propto V$, while $N^m_{IP} \propto V$ and $N^m_{corr} \propto V^{-1}\sqrt{L/a_B}$. Therefore, $\langle i|\mathbf{p}|0\rangle_{IP} \propto V^0$, and $\langle i|\mathbf{p}|0\rangle_{corr} \propto \langle i|\mathbf{p}|0\rangle_{IP}\sqrt{L/a_B}$.

### Intraband matrix element

Intraband transition elements involving two IP states, as in Eq. (4), yield $\langle f|\mathbf{p}|m\rangle \propto k'$. Intraband transition elements involving a correlated intermediate state and final IP state, are obtained from:

$$
\langle \Phi^i_{corr,n}|\frac{d}{dz_2}|\Phi^f_{IP,n}\rangle = ct.\,\frac{a^{1/2}}{L^{3/2}}\,k' \int_{-L/2}^{L/2} \cos^2 kz_1 \cos kz_2 \cos k'z_2\, e^{-a|z_1-z_2|}\, dv. \qquad (22)
$$

Using Eq. (10) identity one obtains:

$$\langle \Phi^i_{corr,n} | \frac{d}{dz_2} | \Phi^f_{IP,n} \rangle =$$
$$ct. \, \frac{a^{1/2}}{L^{3/2}} \, k' \int_{-L/2}^{L/2} \cos^2 k z_1 \int_{-\infty}^{\infty} \frac{1}{2} \, \left[ \cos\left( (k-k') z_2 \right) + \cos\left( (k+k') z_2 \right) \right] \, e^{-a|z_1 - z_2|} \, dz_1 \, dz_2. \tag{23}$$

The two integrals have the same dependence on $L$, which is easily worked out changing variables, $\bar{z}_2 = z_2 - z_1$. For example,

$$\begin{aligned} I &= \int_{-L/2}^{L/2} \cos^2 k z_1 \int_{-\infty}^{\infty} \cos\left( \tilde{k}(z_1 - \bar{z}_2) \right) e^{-a|\bar{z}_2|} \, dz_1 \, d\bar{z}_2 = \\ &= \int_{-L/2}^{L/2} \cos^2 k z_1 \, \cos\left( \tilde{k} z_1 \right) \int_{-\infty}^{\infty} \cos\left( \tilde{k} \bar{z}_2 \right) e^{-a|\bar{z}_2|} \, dz_1 \, d\bar{z}_2 \qquad (24) \\ &\propto L \, \frac{a}{a^2 + \tilde{k}^2} \approx \frac{L}{a} = L \, a_B. \qquad (25) \end{aligned}$$

where we have considered $\tilde{k} \ll a$. Therefore, $\langle \Phi^i_{corr,n} | \frac{d}{dz_2} | \Phi^f_{IP,n} \rangle \propto k' \sqrt{\frac{a_B}{L}}$, a result similar to that of nanoplatelets, but restricted to one dimension.

If the transition is between two correlated states, then:

$$\langle \Phi^i_{corr,n} | \frac{d}{dz_2} | \Phi^f_{corr,n} \rangle = N^i_{corr,\|} \, N^f_{corr,\|} \iint \cos^2 (k z_1) \, \cos(k z_2) \, \frac{d}{dz_2} \, \left( \sin(k' z_2) \, e^{-a|z_2 - z_1|} \right), \tag{26}$$

with $a = 1/a_B + 1/a'_B$. The derivative in Eq. (26) leads to two integrals. The first one (derivative of the sine) is analogous to Eq. (22), except for the normalization constants. The second one (derivative of the exponential) is nearly zero for large $L$ ($k' \to 0$), as it equals $I = 2k'/(4a^2 + k^2)$. Therefore, $\langle \Phi^i_{corr,n} | \frac{d}{dz_2} | \Phi^f_{corr,n} \rangle \propto k' \sqrt{a_B a'_B}/(a_B + a'_B)$.

**Inter-valence-band matrix element**

The transition between to IP states gives $\langle i|f\rangle_{IP-IP} = 1$ if initial and final states have the same quantum numbers, because of envelope function orthonormality. On the other hand, working along the same lines as for intraband transitions (but without derivative in the envelope part), one obtains: $\langle i|f\rangle_{IP-corr} \propto \sqrt{\frac{a_B}{L}}$ and $\langle i|f\rangle_{corr-corr} \propto \frac{\sqrt{a_B\, a'_B}}{(a_B+a'_B)}$.

# Autocorrelation by TPA and second harmonic generation

We briefly discuss the details of the back of the envelope calculation to compare the efficiency of using second harmonic generation (SHG) of a BBO crystal to that of TPA in an auto-correlation measurement of a Ti:Sa laser pulse. As mentioned in the main text we consider a typical 100 fs Ti:Sa laser-pulse at 800 nm wavelength and 100 MHz repetition rate. We take an irradiance of $I_P$=10 GW/cm$^2$ (13 mW CW equivalent power focused by 0.2 NA objective) as reasonable excitation conditions for an SHG auto-correlator with a Rayleigh length of over 10 micron. Following Boyd[2] we calculate the efficiency of the SHG as a function of the interaction length. For TPA we take a dense ensemble of 77x20 nm$^2$ 3.5 monolayer CdSe nanoplatelets (volume fraction of 10 % or 4x10$^{22}$ nanoplatelets per m$^3$) with a TPA cross section of $\sigma^{(2)} = 10^7$ GM.[3] This translates into $\beta$=1.67x10$^{-10}$m/W for the TPA medium consisting of nanoplatelets. Using the non-linear transmission[4] we estimate the efficiency of TPA conversion: $\eta_{TPA} = 1 - 1/(1 + \beta I_P L)$, where $L$ is the interaction length or thickness of our TPA medium. We obtain the following results: For an interaction length of 10 micron, TPA has a 13% efficiency compared to $5{\cdot}10^{-2}$% for a BBO at 800 nm. Even for an extremely short interaction length of 100 nm the TPA autocorrelation exhibits a considerable 0.2% efficiency compared to the vanishing $5{\cdot}10^{-6}$% conversion efficiency of a BBO.

# References


(1) Planelles, J. Simple correlated wave-function for excitons in 0D, quasi-1D and quasi-2D quantum dots. *Theoretical Chemistry Accounts* **2017**, *136*, 81.

(2) Boyd, R. W. *Nonlinear Optics*, 3rd ed.; Academic Press: Burlington, 2008.

(3) Scott, R.; Achtstein, A. W.; Prudnikau, A.; Antanovich, A.; Christodoulou, S.; Moreels, I.; Artemyev, M.; Woggon, U. Two Photon Absorption in II-VI Semiconductors: The Influence of Dimensionality and Size. *Nano Lett.* **2015**, *15*, 4985–4992.

(4) Rumi, M.; Perry, J. W. Two-photon absorption: an overview of measurements and principles. *Adv. Opt. Photonics* **2010**, *2*, 451.
